# Supplementary material for: Sort well with energy-constrained comparisons
Source: arXiv:1610.09223 source file (2016-10-28)
Supplement: Supplementary file 1 [file appendix-123.tex]

\renewcommand{\states}{{
		\Vertex[x=0,y=1,L=$123$]{abc}
		%\node[circle, fill=gray!50] (abc) at (0,1) {$123$};
		\Vertex[L=$321$, x=6.5, y=1]{cba}
		%\node[circle, fill=gray!50] (cba) at (9,1) {$321$};
		\Vertex[L=$213$, x=2, y=2.5]{bac}
		%\node[circle, fill=gray!50] (bac) at (3,2.5) {$213$};
		\Vertex[L=$132$, x=2, y=-.5]{acb}
		%\node[circle, fill=gray!50] (acb) at (3,-.5) {$132$};
		\Vertex[L=$231$, x=4.5, y=2.5]{bca}
		%\node[circle, fill=gray!50] (bca) at (6,2.5) {$231$};
		\Vertex[L=$312$, x=4.5, y=-.5]{cab}
		%\node[circle, fill=gray!50] (cab) at (6,-.5) {$312$};	
	}}
	
	\renewcommand{\abcbac}{{\Edge[label=$-1$](abc)(bac);}}
	\renewcommand{\bacabc}{{\Edge[label=$1$](bac)(abc);}}
	\renewcommand{\abcacb}{{\Edge[label=$-1$](abc)(acb);}}
	\renewcommand{\acbabc}{{\Edge[label=$1$](acb)(abc);}}
	\renewcommand{\bacbca}{{\Edge[label=$-2$](bac)(bca);}}
	\renewcommand{\bcabac}{{\Edge[label=$2$](bca)(bac);}}
	\renewcommand{\bcacba}{{\Edge[label=$-1$](bca)(cba);}}
	\renewcommand{\cbabca}{{\Edge[label=$1$](cba)(bca);}}
	\renewcommand{\cabcba}{{\Edge[label=$-1$](cab)(cba);}}
	\renewcommand{\cbacab}{{\Edge[label=$1$](cba)(cab);}}
	\renewcommand{\cabacb}{{\Edge[label=$2$](cab)(acb);}}
	\renewcommand{\acbcab}{{\Edge[label=$-1$](acb)(cab);}}
	\renewcommand{\acbbca}{{\Edge[label=$-1$, style={bend left = 40}
			](acb)(bca);}}
	\renewcommand{\bcaacb}{{\Edge[label=$1$, style={bend left = 40}
			](bca)(acb);}}
	\renewcommand{\abccba}{{\Edge[label=$-2$](abc)(cba);}}
	\renewcommand{\cbaabc}{{\Edge[label=$2$](cba)(abc);}}
	\renewcommand{\baccab}{{\Edge[label=$-1$, style={bend left = 40}
			](bac)(cab);}}
	\renewcommand{\cabbac}{{\Edge[label=$1$, style={bend left = 40}
			](cab)(bac);}}

	\section{Sorting 123}
	\label{sec:sort-123}
	In this appendix we give a numeric example for the proof of Lemma \ref{le:ratios-abc} with the three elements 1, 2, and 3. We basically show how to pairwise match the good and bad trees.	
	
	\paragraph{The $(123)$ vs $(213)$ case. }
	Figure~\ref{fig:1bacabc} shows all paths between these two states.
	The bad case is \ref{fig:1bacabc:4}, where the ratio between the path and its reversal is $\lambda^4$ which is strictly larger than $\lambda^2=\frac{\pi_{adj}(123)}{\pi_{adj}(213)}$. We will match each bad tree to a good tree containing path \ref{fig:1bacabc:2}.
	
	\begin{lemma}\label{lemma}
		There exists a one-to-one matching from each tree $\overline T$ containing the path  \ref{fig:1bacabc:4} with a tree $\underline T$ containing the path   \ref{fig:1bacabc:2} such that  
		\begin{equation}\label{eq:matching-properties}
			\frac{\P(\overline T)}{\P(\underline T')} =	\frac{\P(\underline T)}{\P(\overline T')} = \lambda^2 \enspace .
		\end{equation}
	\end{lemma}
	
	\begin{proof}
		The matching is shown in Figures~\ref{fig:matching:partI}-\ref{fig:matching:partII}: To check the required identity, observe that $\overline T$ consists of the path \subref{fig:1bacabc:4} of length 2 plus a set of edges of total length $W$, while $\underline T$ has the path \subref{fig:1bacabc:2} plus another set of edges of the same total length $W$, and path \subref{fig:1bacabc:2} has length $0$. Furthermore, the multisets of $\overline T$ and $\underline T$ are equal, i.e., $M(\overline T) = M(\underline T)$. This implies 
		\begin{align*}
			\P(\overline T) =  \lambda^2 \cdot \frac{\lambda^W}{M(\overline T)}& & \P(\overline T') = \lambda^{-2} \cdot \frac{\lambda^W}{M(\overline T)}&  & \P(\underline T) =  \frac{\lambda^W}{M(\underline T)} =  \P(\underline T') \enspace .
		\end{align*}
		which yields \eqref{eq:matching-properties}.
	\end{proof}

	\paragraph{The $(213)$ vs $(231)$ case. }
	Figure~\ref{fig:1bcabac} shows all paths between these two states. There is no bad case, since the ratio between all paths and their reversals is smaller or equal to $\lambda^4=\frac{\pi_{adj}(213)}{\pi_{adj}(231)}$.

	\paragraph{The other cases. }
	The $s=(231)$ vs $s'=(321)$ case is similar to the first case. We can again find pairs of good and bad trees such that the probability ratio between a tree and the reversal of its paired tree is $\lambda^2 = \frac{\pi_{adj}(231)}{\pi_{adl}(321)}$.
	
	The analysis for all other pairs of states $s$ and $s'$ is either analogue to one of the three cases above or any linear combination of them. One can also match the trees to show that the two states $(213)$ and $(132)$ have the same stationary probabilities, or one can match the according trees to show directly that $\frac{\pi_{any}(123)}{\pi_{any}(321)} < \frac{\pi_{adj}(123)}{\pi_{adl}(321)}$.
	
	\begin{figure}
		\begin{subfigure}[b]{0.32\textwidth}
			\centering
			\resizebox{\linewidth}{!}{
				\begin{tikzpicture}
				\states
				
				\bacabc
				\end{tikzpicture}
			}
			\caption{}
			\label{fig:1bacabc:1}
		\end{subfigure}
		\begin{subfigure}[b]{0.32\textwidth}
			\centering
			\resizebox{\linewidth}{!}{
				\begin{tikzpicture}
				\states
				
				\bacbca \bcaacb \acbabc
				\end{tikzpicture}
			}
			\caption{}   
			\label{fig:1bacabc:2}
		\end{subfigure}
		\begin{subfigure}[b]{0.32\textwidth}
			\centering
			\resizebox{\linewidth}{!}{
				\begin{tikzpicture}
				\states
				
				\baccab \cabcba \cbabca \bcaacb \acbabc
				\end{tikzpicture}
			}
			\caption{}
			\label{fig:1bacabc:3}
		\end{subfigure}
		
		\begin{subfigure}[b]{0.32\textwidth}
			\centering
			\resizebox{\linewidth}{!}{
				\begin{tikzpicture}
				\states
				
				\baccab \cabacb \acbabc
				\end{tikzpicture}
			}
			\caption{}
			\label{fig:1bacabc:4}
		\end{subfigure}
		\begin{subfigure}[b]{0.32\textwidth}
			\centering
			\resizebox{\linewidth}{!}{
				\begin{tikzpicture}
				\states
				
				\bacbca \bcacba \cbacab \cabacb \acbabc
				\end{tikzpicture}
			}
			\caption{}
			\label{fig:1bacabc:5}
		\end{subfigure}
		\begin{subfigure}[b]{0.32\textwidth}
			\centering
			\resizebox{\linewidth}{!}{
				\begin{tikzpicture}
				\states
				
				\bacbca \bcacba \cbaabc
				\end{tikzpicture}
			}
			\caption{}
			\label{fig:1bacabc:6}
		\end{subfigure}
		\begin{subfigure}[b]{0.32\textwidth}
			\centering
			\resizebox{\linewidth}{!}{
				\begin{tikzpicture}
				\states
				
				\baccab \cabacb \acbbca \bcacba \cbaabc
				\end{tikzpicture}
			}
			\caption{}
			\label{fig:1bacabc:7}
		\end{subfigure}
		\begin{subfigure}[b]{0.32\textwidth}
			\centering
			\resizebox{\linewidth}{!}{
				\begin{tikzpicture}
				\states
				
				\baccab \cabcba \cbaabc
				\end{tikzpicture}
			}
			\caption{}
			\label{fig:1bacabc:8}
		\end{subfigure}
		\begin{subfigure}[b]{0.32\textwidth}
			\centering
			\resizebox{\linewidth}{!}{
				\begin{tikzpicture}
				\states
				
				\bacbca \bcaacb \acbcab \cabcba \cbaabc
				\end{tikzpicture}
			}
			\caption{}
			\label{fig:1bacabc:9}
		\end{subfigure}
		
		\caption{All paths from (213) to (123).} 
		\label{fig:1bacabc}
	\end{figure}

		\begin{figure}
			\begin{subfigure}[b]{0.32\textwidth}
				\centering
				\resizebox{\linewidth}{!}{
					\begin{tikzpicture}
					\states
					
					\bcabac
					\end{tikzpicture}
				}
				\caption{}
				\label{fig:1bcabac:1}
			\end{subfigure}
			\begin{subfigure}[b]{0.32\textwidth}
				\centering
				\resizebox{\linewidth}{!}{
					\begin{tikzpicture}
					\states
					
					\bcaacb \acbabc \abcbac
					\end{tikzpicture}
				}
				\caption{}   
				\label{fig:1bcabac:2}
			\end{subfigure}
			\begin{subfigure}[b]{0.32\textwidth}
				\centering
				\resizebox{\linewidth}{!}{
					\begin{tikzpicture}
					\states
					
					\bcaacb \acbabc \abccba \cbacab \cabbac
					\end{tikzpicture}
				}
				\caption{}
				\label{fig:1bcabac:3}
			\end{subfigure}
			
			\begin{subfigure}[b]{0.32\textwidth}
				\centering
				\resizebox{\linewidth}{!}{
					\begin{tikzpicture}
					\states
					
					\bcaacb \acbcab \cabbac
					\end{tikzpicture}
				}
				\caption{}
				\label{fig:1bcabac:4}
			\end{subfigure}
			\begin{subfigure}[b]{0.32\textwidth}
				\centering
				\resizebox{\linewidth}{!}{
					\begin{tikzpicture}
					\states
					
					\bcaacb \acbcab \cabcba \cbaabc \abcbac
					\end{tikzpicture}
				}
				\caption{}
				\label{fig:1bcabac:5}
			\end{subfigure}
			\begin{subfigure}[b]{0.32\textwidth}
				\centering
				\resizebox{\linewidth}{!}{
					\begin{tikzpicture}
					\states
					
					\bcacba \cbaabc \abcbac
					\end{tikzpicture}
				}
				\caption{}
				\label{fig:1bcabac:6}
			\end{subfigure}
			\begin{subfigure}[b]{0.32\textwidth}
				\centering
				\resizebox{\linewidth}{!}{
					\begin{tikzpicture}
					\states
					
					\bcacba \cbaabc \abcacb \acbcab \cabbac
					\end{tikzpicture}
				}
				\caption{}
				\label{fig:1bcabac:7}
			\end{subfigure}
			\begin{subfigure}[b]{0.32\textwidth}
				\centering
				\resizebox{\linewidth}{!}{
					\begin{tikzpicture}
					\states
					
					\bcacba \cbacab \cabbac
					\end{tikzpicture}
				}
				\caption{}
				\label{fig:1bcabac:8}
			\end{subfigure}
			\begin{subfigure}[b]{0.32\textwidth}
				\centering
				\resizebox{\linewidth}{!}{
					\begin{tikzpicture}
					\states
					
					\bcacba \cbacab \cabacb \acbabc \abcbac
					\end{tikzpicture}
				}
				\caption{}
				\label{fig:1bcabac:9}
			\end{subfigure}
			
			\caption{All paths from (231) to (213).} 
			\label{fig:1bcabac}
		\end{figure}
	
	\begin{figure}
		\centering
		\begin{minipage}[b]{0.4\textwidth}
			\centering
			\resizebox{\linewidth}{!}{
				\begin{tikzpicture}
				\states
				
				\baccab \cabacb \acbabc \cbabca \bcabac
				\end{tikzpicture}
			}
			\label{fig:match-bacabc:1}
		\end{minipage}
		\begin{minipage}[b]{0.4\textwidth}
			\centering
			\resizebox{\linewidth}{!}{
				\begin{tikzpicture}
				\states
				
				\bacbca \bcaacb \acbabc \cbacab \cabacb
				\end{tikzpicture}
			}  
			\label{fig:match-bacabc:1m}
		\end{minipage}

		\begin{minipage}[b]{0.4\textwidth}
			\centering
			\resizebox{\linewidth}{!}{
				\begin{tikzpicture}
				\states
				
				\baccab \cabacb \acbabc \cbacab \bcabac
				\end{tikzpicture}
			}
			\label{fig:match-bacabc:2}
		\end{minipage}
		\begin{minipage}[b]{0.4\textwidth}
			\centering
			\resizebox{\linewidth}{!}{
				\begin{tikzpicture}
				\states
				
				\bacbca \bcaacb \acbabc \cbabca \cabacb
				\end{tikzpicture}
			}   
			\label{fig:match-bacabc:2m}
		\end{minipage}

		\begin{minipage}[b]{0.4\textwidth}
			\centering
			\resizebox{\linewidth}{!}{
				\begin{tikzpicture}
				\states
				
				\baccab \cabacb \acbabc \cbacab \bcacba
				\end{tikzpicture}
			}
			\label{fig:match-bacabc:3}
		\end{minipage}
		\begin{minipage}[b]{0.4\textwidth}
			\centering
			\resizebox{\linewidth}{!}{
				\begin{tikzpicture}
				\states
				
				\bacbca \bcaacb \acbabc \cbabca \cabcba
				\end{tikzpicture}
			}   
			\label{fig:match-bacabc:3m}
		\end{minipage}
		
		\begin{minipage}[b]{0.4\textwidth}
			\centering
			\resizebox{\linewidth}{!}{
				\begin{tikzpicture}
				\states
				
				\baccab \cabacb \acbabc \cbaabc \bcaacb
				\end{tikzpicture}
			}
			\label{fig:match-bacabc:4}
		\end{minipage}
		\begin{minipage}[b]{0.4\textwidth}
			\centering
			\resizebox{\linewidth}{!}{
				\begin{tikzpicture}
				\states
				
				\bacbca \bcaacb \acbabc \cbaabc \cabbac
				\end{tikzpicture}
			}   
			\label{fig:match-bacabc:4m}
		\end{minipage}		
		\caption{Matching trees with path \subref{fig:bacabc:4} with trees with path \subref{fig:bacabc:2} (part~I).}\label{fig:matching:partI}
	\end{figure}
	
	\begin{figure}\centering
		\begin{minipage}[b]{0.4\textwidth}
			\centering
			\resizebox{\linewidth}{!}{
				\begin{tikzpicture}
				\states
				
				\baccab \cabacb \acbabc \cbabca \bcaacb
				\end{tikzpicture}
			}
			\label{fig:match-bacabc:5}
		\end{minipage}
		\begin{minipage}[b]{0.4\textwidth}
			\centering
			\resizebox{\linewidth}{!}{
				\begin{tikzpicture}
				\states
				
				\bacbca \bcaacb \acbabc \cbabca \cabbac
				\end{tikzpicture}
			}   
			\label{fig:match-bacabc:5m}
		\end{minipage}		
		
		\begin{minipage}[b]{0.4\textwidth}
			\centering
			\resizebox{\linewidth}{!}{
				\begin{tikzpicture}
				\states
				
				\baccab \cabacb \acbabc \cbacab \bcaacb
				\end{tikzpicture}
			}
			\label{fig:match-bacabc:6}
		\end{minipage}
		\begin{minipage}[b]{0.4\textwidth}
			\centering
			\resizebox{\linewidth}{!}{
				\begin{tikzpicture}
				\states
				
				\bacbca \bcaacb \acbabc \cbacab \cabbac
				\end{tikzpicture}
			}   
			\label{fig:match-bacabc:6m}
		\end{minipage}	
		
		\begin{minipage}[b]{0.4\textwidth}
			\centering
			\resizebox{\linewidth}{!}{
				\begin{tikzpicture}
				\states
				
				\baccab \cabacb \acbabc \cbaabc \bcabac
				\end{tikzpicture}
			}
			\label{fig:match-bacabc:7}
		\end{minipage}
		\begin{minipage}[b]{0.4\textwidth}
			\centering
			\resizebox{\linewidth}{!}{
				\begin{tikzpicture}
				\states
				
				\bacbca \bcaacb \acbabc \cbaabc \cabacb
				\end{tikzpicture}
			}   
			\label{fig:match-bacabc:7m}
		\end{minipage}

		\begin{minipage}[b]{0.4\textwidth}
			\centering
			\resizebox{\linewidth}{!}{
				\begin{tikzpicture}
				\states
				
				\baccab \cabacb \acbabc \cbaabc \bcacba
				\end{tikzpicture}
			}
			\label{fig:match-bacabc:8}
		\end{minipage}
		\begin{minipage}[b]{0.4\textwidth}
			\centering
			\resizebox{\linewidth}{!}{
				\begin{tikzpicture}
				\states
				
				\bacbca \bcaacb \acbabc \cabcba \cbaabc
				\end{tikzpicture}
			}   
			\label{fig:match-bacabc:8m}
		\end{minipage}		
		\caption{Matching trees with path \subref{fig:bacabc:4} with trees with path \subref{fig:bacabc:2} (part~II).}
		\label{fig:matching:partII}
	\end{figure}
